# Supplementary material for: Instruct2Act: Mapping Multi-modality Instructions to Robotic Actions with Large Language Model
Source: arXiv:2305.11176 source file (2023-05-24)
Supplement: Supplementary file 1 [file appendix.pdf]

## A Appendix

### A.1 Full Prompts in Instruct2Act

```
1 THIRD PARTY TOOLS:
2 -----
3 You have access to the following tools:
4
5 # Libraries
6 from PIL import Image
7 import numpy as np
8 import scipy
9 import torch
10 import cv2
11 import math
12 from typing import Union
13
14 IMPLEMENTED TOOLS:
15 -----
16 You have access to the following tools:
17
18 # First Level: File IO
19 templates = {} # dictionary to store and cache the multi-modality instruction
20 # possible keys in templates: "scene", "dragged_obj", "base_obj"
21 # NOTE: the word in one instruction inside {} stands for the visual part of the
22 # instruction and will be obtained with get operation
23 # Example: {scene} -> templates.get('scene')
24 BOUNDS = {} # dictionary to store action space boundary
25
26 def GetObsImage(obs) -> Image.Image:
27     """Get the current image to start the system.
28     Examples:
29         image = GetObsImage(obs)
30     """
31     pass
32
33 def SaveFailureImage() -> str:
34     """Save images when execution fails
35     Examples:
36         info = SaveFailureImage()
37     """
38     pass
39
40 # Second Level: Core Modules
41 ## Perception Modules
42 def SAM(image: Image.Image) -> dict:
43     """Get segmentation results with SAM
44     Examples:
45         masks = SAM(image=image)
46     """
47     pass
48
49 def ImageCrop(image: Image.Image, masks: dict):
50     """Crop image with given masks
51     Examples:
52         objs, masks = ImageCrop(image=image, masks=masks)
53     """
54     pass
55
56 def CLIPRetrieval(objs: list, query: str | Image.Image, pre_obj1: int = None, pre_obj2:
57     int = None) -> np.ndarray:
58     """Retrieve the desired object(s) with CLIP, the query could be string or an image
59     Examples:
60         obj_0 = CLIPRetrieval(objs=objs, query='the yellow and purple polka dot pan') #
61         the query is a string
62         obj_0 = CLIPRetrieval(objs=objs, query=templates['dragged_obj']) # the query is
63         image, stored in templates
64     """
65     pass
66
67 def get_objs_match(objs_list1: list, objs_list2: list) -> tuple:
68     """Get correspondences of objects between two lists using the Hungarian Algorithm"""
69     return (list, list)
70
71 ## Action Modules
72 def Pixel2Loc(obj: np.ndarray, masks: np.ndarray) -> np.ndarray:
73     """Map masks to specific locations"""
74     pass
```

```

72 def PickPlace(pick: np.ndarray, place: np.ndarray, bounds: np.ndarray, yaw_angle_degree:
    float = None, tool: str = "suction") -> str:
73     """Pick and place the object based on given locations and bounds"""
74     pass
75
76 def DistractorActions(mask_obs: list, obj_list: list, tool: str = "suction") -> list:
77     """Remove observed objects that conflict with the goal object list"""
78     pass
79
80 def RearrangeActions(pick_masks: list, place_masks: list, pick_ind: list, place_ind: list
    , bounds: np.ndarray, tool: str = "suction") -> list:
81     """Composite multiple pick and place actions"""
82     pass
83
84 # Third Level: Connect to Robotic Hardware
85 def RobotExecution(action) -> dict
86     """Execute the robot, then return the execution result as a dict """
87     pass
88
89 Examples:
90 -----
91 Use the following examples to understand tools:
92 ## Example 1
93 # Instruction: Put the checkerboard round into the yellow and purple polka dot pan.
94 def main_1() -> dict:
95     """Execute the given instructions of placing the checkerboard round into the yellow
    and purple polka dot pan"""
96     image = GetObsImage(obs)
97     masks = SAM(image=image)
98     objs, masks = ImageCrop(image=image, masks=masks)
99     obj_0 = CLIPRetrieval(objs=objs, query='the yellow and purple polka dot pan')
100     loc_0 = Pixel2Loc(obj=obj_0, masks=masks)
101     obj_1 = CLIPRetrieval(objs=objs, query='the checkerboard round', pre_obj1=obj_0)
102     loc_1 = Pixel2Loc(obj=obj_1, masks=masks)
103     action = PickPlace(pick=loc_1, place=loc_0, bounds=BOUNDS)
104     info = RobotExecution(action=action)
105     return info
106
107 ## Example 2:
108 # Instruction: Rotate the {dragged_obj} 150 degrees.
109 def main_2() -> dict:
110     """Execute the given instructions of rotating the {dragged_obj} 150 degrees"""
111     image = GetObsImage(obs)
112     masks = SAM(image=image)
113     objs, masks = ImageCrop(image=image, masks=masks)
114     obj_0 = CLIPRetrieval(objs=objs, query=templates.get("dragged_obj"))
115     loc_0 = Pixel2Loc(obj=obj_0, masks=masks)
116     action = PickPlace(pick=loc_0, place=loc_0, bounds=BOUNDS, yaw_angle_degree=150)
117     info = RobotExecution(action=action)
118     return info
119
120 ## Example 3
121 # Instruction: Rearrange to this {scene} then restore.
122 # Note: for RESTORE operation, direct conduct an inverse operation
123 def main_3() -> dict:
124     """Execute the given instructions of rearranging the objects to match the objects in
    the given scene"""
125     image_obs = GetObsImage(obs)
126     image_goal = templates.get("scene")
127     masks_obs = SAM(image=image_obs)
128     objs_obs, masks_obs = ImageCrop(image=image_obs, masks=masks_obs)
129     masks_goal = SAM(image=image_goal)
130     objs_goal, masks_goal = ImageCrop(image=image_goal, masks=masks_goal)
131     row, col = get_objs_match(objs_list1=objs_goal, objs_list2=objs_obs)
132     action_1 = DistractorActions(mask_obs=masks_obs, obj_list=col)
133     action_2 = RearrangeActions(pick_masks=masks_obs, place_masks=masks_goal, pick_ind=
    col, place_ind=row, bounds=BOUNDS)
134     action_3 = RearrangeActions(pick_masks=masks_goal, place_masks=masks_obs, pick_ind=
    row, place_ind=col, bounds=BOUNDS)
135     actions = []
136     actions.extend(action_1).extend(action_2).extend(action_3)
137     info = RobotExecution(action=actions)
138     return info
139
140
141 ## Example 4
142 # Instruction: Put the yellow and blue stripe object in {scene} into the orange object.
143 def main_4() -> dict:
144     """Execute the given instructions of placing the yellow and blue stripe object in
    scene into the orange object"""
145     image = GetObsImage(obs)

```

```

146 masks_obs = SAM(image=image)
147 objs_goal, masks_goal = ImageCrop(image=templates['scene'], masks=SAM(image=templates
    ['scene']))
148 goal = CLIPRetrieval(objs=objs_goal, query='the yellow and blue stripe object')
149 target = CLIPRetrieval(objs=objs_obs, query=objs_goal[goal])
150 loc_0 = Pixel2Loc(obj=target, masks=masks_obs)
151 obj_1 = CLIPRetrieval(objs=objs_obs, query='the orange object', pre_obj1=target)
152 loc_1 = Pixel2Loc(obj=obj_1, masks=masks_obs)
153 action = PickPlace(pick=loc_0, place=loc_1, bounds=BOUNDS)
154 info = RobotExecution(action=action)
155 return info
156
157 ## Example 5
158 # Instruction: Put the {dragged_obj} into the {base_obj_1} then {base_obj_2}. Finally
    restore it into its original container.
159 def mian_5() -> dict:
160     masks = SAM(obs_image)
161     objs, masks = ImageCrop(obs_image, masks)
162     base_obj_1 = CLIPRetrieval(objs, templates['base_obj_1'])
163     base_obj_2 = CLIPRetrieval(objs, templates['base_obj_2'], pre_obj1=base_obj_1)
164     dragged_obj = CLIPRetrieval(objs, templates['dragged_obj'], pre_obj1=base_obj_1,
        pre_obj2=base_obj_2)
165     loc_base_obj_1 = Pixel2Loc(base_obj_1, masks)
166     loc_base_obj_2 = Pixel2Loc(base_obj_2, masks)
167     loc_dragged_obj = Pixel2Loc(dragged_obj, masks)
168
169     action_1 = PickPlace(pick=loc_dragged_obj, place=loc_base_obj_1, bounds=BOUNDS)
170     action_2 = PickPlace(pick=loc_base_obj_1, place=loc_base_obj_2, bounds=BOUNDS)
171     action_3 = PickPlace(pick=loc_base_obj_2, place=loc_dragged_obj, bounds=BOUNDS)
172     actions = [action_1, action_2, action_3]
173
174     info = RobotExecution(action=actions)
175     return info
176
177 Begin to execute the task:
178 -----
179 Please solve the following instruction step-by-step. You should implement the main()
    function and output in the Python-code style.
180
181 Instruction: INSERT INSTRUCTION HERE.

```

Listing 1: An example of a full prompt in Instruct2Act

## A.2 Processing Module in Instruct2Act

When pre-trained models are utilized directly on downstream tasks without any fine-tuning, they inevitably suffer from problems like incompleteness or incorrectness. In light of this, it is advisable to insert processing modules or adapters between the output of the large model and the downstream tasks which can effectively tackle the issues caused by this zero-shot paradigm. The entire loop of execution for robot tasks comprises three modules, namely, perception, planning, and execution. We have curated various processing programs for each of these modules designed for tabletop manipulation domains.

**Image Pre-Processing** In the case of zero-shot SAM outputs, a significant challenge is distinguishing the target object from shadow regions that might appear within the image. As object shadows cannot be grasped, their presence poses additional difficulty for robot grasping tasks. Furthermore, tabletop manipulation domains typically involve camera placement above the robotic arm, leading to large shadows cast onto the operating table. To account for this, we adopted a simple yet efficient image preprocessing methodology: to mitigate the effect of shadows, we employed the gray threshold filter followed by the close morphological operation to fill in small gaps that the filter might produce.

**Mask Post-Processing** In the zero-shot setting, it is observed that the SAM produces multiple segments (e.g. masks) that may be discontinuous or discrete. There may also be detected objects with missing parts, or holes inside, as shown in Fig 6-C. These misleading semantic mask outputs will inevitably confuse the subsequent modules and greatly challenge the robot grasping task. In order to address the given problem, we have developed a set of processing modules to work with the SAM output. The modules include the following methods:

- We apply a filtering process on the output based on the mask’s size. This process removes any output that is clearly not part of the target object. Such output may include objects that cannot be moved, like tables or patterns on the target object.

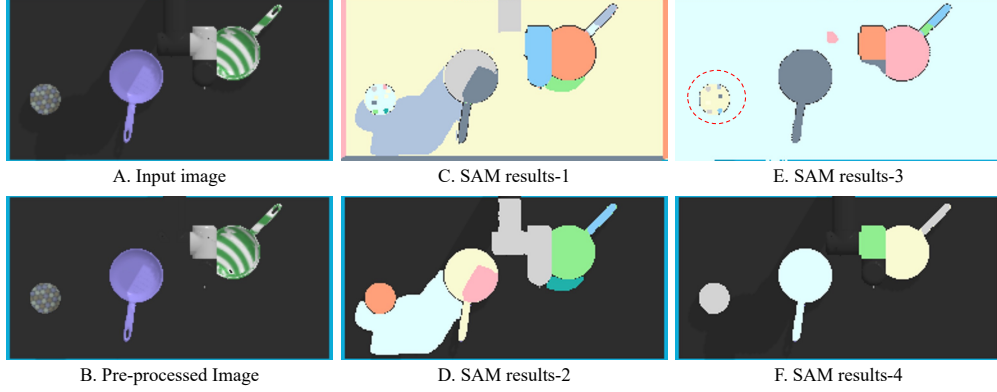

Figure 6: The segmentation outputs w / wo the processing methods. Figure A is the original image which is produced by a top-down camera. Figure B is the image with the proposed image pre-processing pipeline. Figure-  $\{C, D, E, F\}$  are the SAM results directly on the original image, only with the mask post-processing, only with image pre-processing, and with both processing modules respectively. The portion highlighted by the red circle demonstrates the redundant output of the SAM without additional processing applied to a texture object.

| Instruction Modal                      | Task 01 | Task 03 |
|----------------------------------------|---------|---------|
| Pointing-Language Enhanced Instruction | 90.7    | 98.0    |

Table 6: Results with pointing-language enhanced instruction.

- A dilation operation is used to effectively eliminate unrealistic small holes or unconnected gaps. To avoid significant changes to the mask’s size due to dilation, we then use an erosion operation. These two procedures combine to create what is known as the opening morphological operation.
- In some instances where there are multiple segmentation outputs for a single object, we employ the Non-Maximum Suppression (NMS) operator to reduce redundant mask output.

### A.3 Pointing-Language Enhanced Instruction

When utilizing the pointing-language mode of Instruct2Act, the system will display the initial task instruction and observation image. Next, the user will select the target objects by clicking on them with the cursor. These click points will then act as point prompts to guide the SAM’s segmentation process. We evaluated this mode on Task 01 and Task 03, averaging the results over 150 instances with one seed.

Table 6 shows that our Instruct2Act achieves better results with the pointing-language enhanced mode than with the pure-language instruction mode. This could be due to the stronger prior information provided by the user’s click operations.

### A.4 Evaluation Task Description

**Simple object manipulation.** The agent is asked to follow the basic instructions to take action.

- **Visual Manipulation.** The agent is required to pick a specific object and place it into a specified container. The agent needs to first recognize the target objects aligning with the task instruction specified by the natural language description or by the image pattern.

- Scene Understanding. The agent must first identify the target object with the described texture by grounding the natural language description and the scene image simultaneously and then put the target object into the container with a specific color.
- Rotation. The agent is required to rotate a specific object by certain degrees along the z-axis.

**Visual goal-reaching.** The agent is asked to manipulate the objects to match the goal states described by the goal scene image,

- Rearrange. The agent is required to rearrange the target objects to reach the goal configuration. The agent needs to identify the possible existing distractors and move them away to avoid position conflicts.
- Rearrange then restore. The agent is required to restore the object placements after the rearrangement operations.

**Visual Reasoning** The agent is asked to make decisions and take actions where reasoning and memory ability are required.

- Pick in order then restore. The agent is required to pick and place the target object sequentially into different containers and finally restore it to the initial container.

VIMABench [15] presents a 4-level evaluation protocol that progressively increases in difficulty for trained agents. Our experiments utilize the first 3 levels of this protocol, which test the generalization abilities of our agents. Level 1 (L1) placement generalization randomly arranges the placement of target objects, whereas L2 combinatorial generalization generates new combinations of target materials and object descriptions. Finally, L3 novel object generalization tests our agents’ ability to generalize to novel materials and objects.

## A.5 Ablation Studies on Prompt Element

We use the same task instruction *Put the polka dot block into the green container.* for all experiments here. Because the outputs of LLMs are somewhat random, we will display the results of three consecutive outputs.

```

1 def main():
2     # Step 1: Get the current observation image
3     image = GetObsImage(obs)
4
5     # Step 2: Segment the image to get masks
6     masks = SAM(image=image)
7
8     # Step 3: Crop the image based on masks
9     objs, masks = ImageCrop(image=image, masks=masks)
10
11    # Step 4: Retrieve the object(s) of interest using CLIP
12    query = 'polka dot block' # define the query
13    polka_dot_block = CLIPRetrieval(objs=objs, query=query)
14
15    # Step 5: Map masks to specific object locations
16    obj_loc = Pixel2Loc(obj=polka_dot_block, masks=masks)
17
18    # Step 6: Get the pick and place locations and action boundaries
19    pick_loc = obj_loc # we want to pick up the polka dot block
20    place_loc = BOUNDS['green_container'] # the green container is the place location
21    bounds = BOUNDS['PickPlace_bounds'] # limits of the pick and place action
22
23    # Step 7: Perform any necessary distracting actions
24    obj_list = ['polka dot block'] # define the goal object list
25    masks_obs = np.delete(masks, polka_dot_block, axis=0) # remove the polka dot block
26    DistractorActions = DistractorActions(mask_obs=masks_obs, obj_list=obj_list)
27
28    # Step 8: Plan and execute the pick and place action
29    pick_masks = masks[polka_dot_block]
30    pick_ind = [0] # We only want to pick up one object
31    place_masks = np.expand_dims(place_loc, axis=0) # expand dims to match the pick loc
32    place_ind = [0] # We only have one object to place
33    action_seq = RearrangeActions(pick_masks=pick_masks, place_masks=place_masks,
34                                  pick_ind=pick_ind, place_ind=place_ind, bounds=bounds)

```

```

34 action_seq = DistractorActions + action_seq # combine distractor actions with pick
    and place actions
35 for action in action_seq:
36     result = RobotExecution(action)
37     time.sleep(result['time_elapsed']) # wait for the robot to finish the action
38 return result

```

Listing 2: Generation with Only API Definition provided in Prompt. First Trial

```

1 def main():
2     # Step 1: Get the current observation image
3     obs_image = GetObsImage(obs)
4
5     # Step 2: Use SAM to get segmentation results
6     masks = SAM(image=obs_image)
7
8     # Step 3: Crop the image to get object bounding boxes
9     objs, masks = ImageCrop(image=obs_image, masks=masks)
10
11    # Step 4: Use CLIP to retrieve the polka dot block
12    polka_dot = CLIPRetrieval(objs=objs, query='polka dot block')
13
14    # Step 5: Use CLIP to retrieve the green container
15    green_container = CLIPRetrieval(objs=objs, query='green container')
16
17    # Step 6: Map masks to specific locations
18    polka_dot_loc = Pixel2Loc(obj=polka_dot, masks=masks)
19    green_container_loc = Pixel2Loc(obj=green_container, masks=masks)
20
21    # Step 7: Pick and place the polka dot into the green container
22    action = PickPlace(pick=polka_dot_loc, place=green_container_loc, bounds=BOUNDS)
23
24    # Step 8: Execute the action using the robotic hardware
25    result = RobotExecution(action)
26
27    # Step 9: Save images if execution fails
28    if not result['success']:
29        SaveFailureImage()
30
31    # Step 10: return the result
32    return result

```

Listing 3: Generation with Only API Definition provided in Prompt. Second Trial

```

1 def main():
2     # Step 1: Get the current observation image
3     obs_image = GetObsImage(obs)
4
5     # Step 2: Use SAM to get segmentation results
6     masks = SAM(image=obs_image)
7
8     # Step 3: Crop the image to get object bounding boxes
9     objs, masks = ImageCrop(image=obs_image, masks=masks)
10
11    # Step 4: Use CLIP to retrieve the polka dot block
12    polka_dot = CLIPRetrieval(objs=objs, query='polka dot block')
13
14    # Step 5: Use CLIP to retrieve the green container
15    green_container = CLIPRetrieval(objs=objs, query='green container')
16
17    # Step 6: Map masks to specific locations
18    polka_dot_loc = Pixel2Loc(obj=polka_dot, masks=masks)
19    green_container_loc = Pixel2Loc(obj=green_container, masks=masks)
20
21    # Step 7: Pick and place the polka dot into the green container
22    action = PickPlace(pick=polka_dot_loc, place=green_container_loc, bounds=BOUNDS)
23
24    # Step 8: Execute the action using the robotic hardware
25    result = RobotExecution(action)
26
27    # Step 9: Save images if execution fails
28    if not result['success']:
29        SaveFailureImage()
30
31    # Step 10: Print the result
32    print(result)

```

Listing 4: Generation with Only API Definition provided in Prompt. Third Trial

```

1 def main() -> dict:
2     """Execute the given instructions of placing the polka dot block into the green
3     container"""
4     image = GetObsImage(obs)
5     masks = SAM(image=image)
6     objs, masks = ImageCrop(image=image, masks=masks)
7     obj_0 = CLIPRetrieval(objs=objs, query="the polka dot block")
8     loc_0 = Pixel2Loc(obj=obj_0, masks=masks)
9     obj_1 = CLIPRetrieval(objs=objs, query="the green container")
10    loc_1 = Pixel2Loc(obj=obj_1, masks=masks)
11    action = PickPlace(pick=loc_0, place=loc_1, bounds=BOUNDS)
12    info = RobotExecution(action=action)
13    return info

```

Listing 5: Generation with Only In-Context Examples provided in Prompt. First Trial

```

1 def main() -> dict:
2     # Use object detection to get the object and container locations from the RGB image.
3     image = GetObsImage(obs)
4     masks = SAM(image=image)
5     objs, masks = ImageCrop(image=image, masks=masks)
6     block_obj = CLIPRetrieval(objs=objs, query='the polka dot block')
7     container_obj = CLIPRetrieval(objs=objs, query='the green container')
8
9     # Convert the pixel locations of the objects into robot reference frame (in meters).
10    block_loc = Pixel2Loc(obj=block_obj, masks=masks)
11    container_loc = Pixel2Loc(obj=container_obj, masks=masks)
12
13    # Move the robot's arm to pick and place the block into the container.
14    action = PickPlace(pick=block_loc, place=container_loc, bounds=BOUNDS)
15    info = RobotExecution(action=action)
16    return info

```

Listing 6: Generation with Only In-Context Examples provided in Prompt. Second Trial

```

1 def main() -> dict:
2     """Execute the given instructions of placing the polka dot block into the green
3     container"""
4     # Obtain the image of the scene
5     image = GetObsImage(obs)
6
7     # Segment the image using Semantic Affinity Module (SAM)
8     masks = SAM(image=image)
9
10    # Crop image to obtain individual objects and their masks
11    objs, masks = ImageCrop(image=image, masks=masks)
12
13    # Retrieve the polka dot block object using OpenAI's CLIP model
14    obj_0 = CLIPRetrieval(objs=objs, query='the polka dot block')
15
16    # Get the location of the green container
17    obj_1 = CLIPRetrieval(objs=objs, query='the green container')
18    loc_1 = Pixel2Loc(obj=obj_1, masks=masks)
19
20    # Move the polka dot block from its current location to the green container
21    loc_0 = Pixel2Loc(obj=obj_0, masks=masks)
22    action = PickPlace(pick=loc_0, place=loc_1, bounds=BOUNDS)
23    info = RobotExecution(action=action)
24
25    # Return the execution information
26    return info

```

Listing 7: Generation with Only In-Context Examples provided in Prompt. Third Trial

```

1 def main() -> dict:
2     # first, capture an image of the current scene
3     image = GetObsImage(obs)
4
5     # generate object masks using the SAM module
6     masks = SAM(image=image)
7
8     # identify the objects in the scene using the masks
9     objs, masks = ImageCrop(image=image, masks=masks)
10
11    # use CLIPRetrieval to find the polka dot block and the green container
12    polka_dot_block = CLIPRetrieval(objs=objs, query="the polka dot block")
13    green_container = CLIPRetrieval(objs=objs, query="the green container")
14
15    # convert the object masks to location coordinates

```

```

16 polka_dot_block_loc = Pixel2Loc(obj=polka_dot_block, masks=masks)
17 green_container_loc = Pixel2Loc(obj=green_container, masks=masks)
18
19 # use the PickPlace function to pick up the polka dot block and place it in the green
   container
20 action = PickPlace(pick=polka_dot_block_loc, place=green_container_loc, bounds=BOUNDS
   )
21
22 # execute the action on the robot using the RobotExecution function and return the
   result
23 info = RobotExecution(action=action)
24 return info

```

Listing 8: Generation with both API Definition and In-context Examples provided in Prompt. First Trial
